# Supplementary material for: Understanding the Double Descent Phenomenon in Deep Learning
Source: arXiv:2403.10459 source file (2024-03-15)
Supplement: Supplementary file 1 [file 5_appendices.tex]

\appendix
\section{Appendices}
